# Supplementary material for: Neural Machine Translation for Mathematical Formulae
Source: arXiv:2305.16433 source file (2023-05-25)
Supplement: Supplementary file 1 [file sm_tables.pdf]

## B Qualitative Analysis – Mathematical Functions Site

This supplementary material presents 8 translation samples from LaTeX to Mathematica. All samples are randomly selected, only restricted by the editorial constraint of fitting on a single page and restricted to have a similar amount of exact matches and erroneous cases. Equations B.1–B.4 are erroneous translations, while Equations B.5–B.8 lead to exact matches.

Here, the LaTeX formulae were generated by Mathematica's export function.

Table 3: Equations including the tokenized LaTeX input, the (optional) interpretation by Mathematica (Mat.), our translation (NMT), and the ground truth (GT.). (NMT+GT.) denotes that our translation is equal to the ground truth.

$$\sigma_k(n) = \prod_{j=1}^{m} \sigma_k\left(p_j^{n_j}\right) /;\text{FactorInteger}[n] = \{\{p_1, n_1\}, \ldots, \{p_m, n_m\}\} \land p_j \in \mathbb{P} \land k \in \mathbb{Z} \land n \in \mathbb{Z} \land n > 0 \quad \text{(B.1)}$$

| | |
|---|---|
| LaTeX | **\sigma _ k ( n )** = \prod _ { j = 1 } ^ m \sigma _ k \left( p _ j ^ { n _ j } \right) \text{/;} \text{FactorInteger} [ n ] = \le f t \{ \le f t \{ p _ 1 , n _ 1 \right \} , \ldots , \le f t \{ p _ m , n _ m \right \} \right \} \land p _ j \in \mathbb{P} \land k \in \mathbb{Z} \land n \in \mathbb{Z} **\land** n > 0 |
| Mat. | **Subscript[\[Sigma], k][n]** == \!\( *UnderoverscriptBox[\(\[Product]\), \(j = 1\), \(m\)]\( \(*SubscriptBox[\(\[Sigma]\), \(k\)]\)[ *SubsuperscriptBox[\(p\), \(j\), SubscriptBox[\(n\), \(j\)]]]\)\) /; FactorInteger[ n] == {{Subscript[p, 1], Subscript[n, 1]}, \[Ellipsis], {Subscript[p, m], Subscript[n, m]}}\[Wedge]Subscript[p, j] \[Element] P\[Wedge]k \[Element] Z\[Wedge]n \[Element] Z**\[Wedge]**n > 0 |
| NMT | **DivisorSigma [ k , n ]** == Product [ DivisorSigma [ k , Subscript [ p , j ] ^ Subscript [ n , j ] , { j , 1 , m } ] /; FactorInteger [ n ] == { { Subscript [ p , 1 ] , Subscript [ n , 1 ] } , \[Ellipsis] , { Subscript [ p , m ] , Subscript [ n , m ] } } && Element [ Subscript [ p , j ] , Primes ] && Element [ k , Integers ] && Element [ n , Integers ] **&&** n > 0 |
| GT. | **DivisorSigma [ k , n ]** == Product [ DivisorSigma [ k , Subscript [ p , j ] ^ Subscript [ n , j ] **]** , { j , 1 , m } ] /; FactorInteger [ n ] == { { Subscript [ p , 1 ] , Subscript [ n , 1 ] } , \[Ellipsis] , { Subscript [ p , m ] , Subscript [ n , m ] } } && Element [ Subscript [ p , j ] , Primes ] && Element [ k , Integers ] && Element [ n , Integers ] **&&** n > 0 |

$$\wp\left(z; g_2, g_3\right) = -\frac{\sigma(z-z_0;g_2,g_3)\sigma(z+z_0;g_2,g_3)}{\sigma(z;g_2,g_3)^2\sigma(z_0;g_2,g_3)^2} /; z_0 = \wp^{-1}\left(0; g_2, g_3\right) \quad \text{(B.2)}$$

| | |
|---|---|
| LaTeX | **\wp** \left( z ; g _ 2 , g _ 3 \right) = - \frac { **\sigma** \left( z - z _ 0 ; g _ 2 , g _ 3 \right) \sigma \left( z + z _ 0 ; g _ 2 , g _ 3 \right) } { \sigma \left( z ; g _ 2 , g _ 3 \right) { } ^ 2 \sigma \left( z _ 0 ; g _ 2 , g _ 3 \right) { } ^ 2 } \text{/;} z _ 0 = **\wp ^ { - 1 }** \left( 0 ; g _ 2 , g _ 3 \right) |
| Mat. | **WeierstrassP**[ z, {Subscript[g, 2], Subscript[g, 3]}] == -((**\[Sigma]**[z - Subscript[z, 0]; Subscript[g, 2], Subscript[g, 3]] \[Sigma][z + Subscript[z, 0]; Subscript[g, 2], Subscript[g, 3]])/(\[Sigma][z; Subscript[g, 2], Subscript[g, 3]] \[Null]^2 \[Sigma][Subscript[z, 0]; Subscript[g, 2], Subscript[g, 3]] \[Null]^2)) /; Subscript[z, 0] == **InverseWeierstrassP**[0, {Subscript[g, 2], Subscript[g, 3]}] |
| NMT | **WeierstrassP** [ z , { Subscript [ g , 2 ] , Subscript [ g , 3 ] } ] == - ( **WeierstrassSigma** [ z - Subscript [ z , 0 ] , { Subscript [ g , 2 ] , Subscript [ g , 3 ] } ] WeierstrassSigma [ z + Subscript [ z , 0 ] , { Subscript [ g , 2 ] , Subscript [ g , 3 ] } ] / ( WeierstrassSigma [ z , { Subscript [ g , 2 ] , Subscript [ g , 3 ] } ] ^ 2 WeierstrassSigma [ Subscript [ z , 0 ] , { Subscript [ g , 2 ] , Subscript [ g , 3 ] } ] ^ 2 ) ) /; Subscript [ z , 0 ] == **InverseWeierstrassP** [ 0 , { Subscript [ g , 2 ] , Subscript [ g , 3 ] } ] |
| GT. | **WeierstrassP** [ z , { Subscript [ g , 2 ] , Subscript [ g , 3 ] } ] == - ( **( WeierstrassSigma** [ z - Subscript [ z , 0 ] , { Subscript [ g , 2 ] , Subscript [ g , 3 ] } ] WeierstrassSigma [ z + Subscript [ z , 0 ] , { Subscript [ g , 2 ] , Subscript [ g , 3 ] } ] **)** / ( WeierstrassSigma [ z , { Subscript [ g , 2 ] , Subscript [ g , 3 ] } ] ^ 2 WeierstrassSigma [ Subscript [ z , 0 ] , { Subscript [ g , 2 ] , Subscript [ g , 3 ] } ] ^ 2 ) ) /; Subscript [ z , 0 ] == **InverseWeierstrassP** [ 0 , { Subscript [ g , 2 ] , Subscript [ g , 3 ] } ] |

Table 3: Equations including the tokenized LaTeX input, the (optional) interpretation by Mathematica (Mat.), our translation (NMT), and the ground truth (GT.). (NMT+GT.) denotes that our translation is equal to the ground truth.

| | |
|---|---|
| | $$Q_4^9(z) = -\frac{\text{<number\_17>}\left(3+\text{<number\_04>}z^2+\text{<number\_21>}z^4\right)}{(z-1)^{9/2}(z+1)^{9/2}} \quad \text{(B.3)}$$ |
| LaTeX | **Q _ 4 ^ 9 ( z )** = - \frac { **<number_17>** \left( 3 + **<number_04>** z ^ 2 + **<number_21>** z ^ 4 \right) } { ( z - 1 ) ^ { 9 / 2 } ( z + 1 ) ^ { 9 / 2 } } |
| NMT | **GammaRegularized** [ 4 , 9 , z ] == - ( ( **<number_17>** ( 3 + **<number_04>** z ^ 2 + **<number_21>** z ^ 4 ) ) / ( ( z - 1 ) ^ ( 9 / 2 ) ( z + 1 ) ^ ( 9 / 2 ) ) ) |
| GT. | **LegendreQ** [ 4 , 9 , 3 , z ] == - ( ( **<number_17>** ( 3 + **<number_04>** z ^ 2 + **<number_21>** z ^ 4 ) ) / ( ( z - 1 ) ^ ( 9 / 2 ) ( z + 1 ) ^ ( 9 / 2 ) ) ) |
| | $$\wp\left(z_1 \pm z_2; g_2, g_3\right) = \frac{\left(\wp(z_1;g_2,g_3)+\wp(z_2;g_2,g_3)\right)\left(2\wp(z_1;g_2,g_3)\wp(z_2;g_2,g_3)-\frac{g_2}{2}\right)-\left(g_3\mp\wp'(z_1;g_2,g_3)\wp'(z_2;g_2,g_3)\right)}{2\left(\wp(z_1;g_2,g_3)-\wp(z_2;g_2,g_3)\right)^2} \quad \text{(B.4)}$$ |
| LaTeX | \wp \left( z _ 1 \pm z _ 2 ; g _ 2 , g _ 3 \right) = \frac { \left( \wp \left( z _ 1 ; g _ 2 , g _ 3 \right) + \wp \left( z _ 2 ; g _ 2 , g _ 3 \right) \right) \left( 2 \wp \left( z _ 1 ; g _ 2 , g _ 3 \right) \wp \left( z _ 2 ; g _ 2 , g _ 3 \right) - \frac { g _ 2 } { 2 } \right) - \left( g _ 3 \mp \wp ' \left( z _ 1 ; g _ 2 , g _ 3 \right) \wp ' \left( z _ 2 ; g _ 2 , g _ 3 \right) \right) } { 2 \left( \wp \left( z _ 1 ; g _ 2 , g _ 3 \right) - \wp \left( z _ 2 ; g _ 2 , g _ 3 \right) \right) { } ^ 2 } |
| NMT | WeierstrassP [ Subscript [ z , 1 ] \[PlusMinus] Subscript [ z , 2 ] , { Subscript [ g , 2 ] , Subscript [ g , 3 ] } ] == ( ( WeierstrassP [ Subscript [ z , 1 ] , { Subscript [ g , 2 ] , Subscript [ g , 3 ] } ] + WeierstrassP [ Subscript [ z , 2 ] , { Subscript [ g , 2 ] , Subscript [ g , 3 ] } ] ) / ( 2 ( WeierstrassP [ Subscript [ z , 1 ] , { Subscript [ g , 2 ] , Subscript [ g , 3 ] } ] WeierstrassP [ Subscript [ z , 2 ] , { Subscript [ g , 2 ] , Subscript [ g , 3 ] } ] - Subscript [ g , 2 ] / 2 ) - ( Subscript [ g , 3 ] , WeierstrassPPrime [ Subscript [ z , 1 ] , { Subscript [ g , 2 ] , Subscript [ g , 3 ] } ] WeierstrassPPrime [ Subscript [ z , 2 ] , { Subscript [ g , 2 ] , Subscript [ g , 3 ] } ] ) ) / ( 2 ( WeierstrassP [ Subscript [ z , 1 ] , { Subscript [ g , 2 ] , Subscript [ g , 3 ] } ] - WeierstrassP [ Subscript [ z , 2 ] , { Subscript [ g , 2 ] , Subscript [ g , 3 ] } ] ) ) |
| GT. | WeierstrassP [ Subscript [ z , 1 ] \[PlusMinus] Subscript [ z , 2 ] , { Subscript [ g , 2 ] , Subscript [ g , 3 ] } ] == ( 1 / ( 2 ( WeierstrassP [ Subscript [ z , 1 ] , { Subscript [ g , 2 ] , Subscript [ g , 3 ] } ] - WeierstrassP [ Subscript [ z , 2 ] , { Subscript [ g , 2 ] , Subscript [ g , 3 ] } ] ) ^ 2 ) ) ( ( WeierstrassP [ Subscript [ z , 1 ] , { Subscript [ g , 2 ] , Subscript [ g , 3 ] } ] + WeierstrassP [ Subscript [ z , 2 ] , { Subscript [ g , 2 ] , Subscript [ g , 3 ] } ] ) ( 2 WeierstrassP [ Subscript [ z , 1 ] , { Subscript [ g , 2 ] , Subscript [ g , 3 ] } ] WeierstrassP [ Subscript [ z , 2 ] , { Subscript [ g , 2 ] , Subscript [ g , 3 ] } ] - ( 1 / 2 ) Subscript [ g , 2 ] ) - ( Subscript [ g , 3 ] \[MinusPlus] WeierstrassPPrime [ Subscript [ z , 1 ] , { Subscript [ g , 2 ] , Subscript [ g , 3 ] } ] WeierstrassPPrime [ Subscript [ z , 2 ] , { Subscript [ g , 2 ] , Subscript [ g , 3 ] } ] ) ) |
| | $$\delta(0,0,0,0) = 1 \quad \text{(B.5)}$$ |
| LaTeX | \delta ( 0 , 0 , 0 , 0 ) = 1 |
| Mat. | \[Delta][0, 0, 0, 0] == 1 |
| NMT+GT. | DiscreteDelta [ 0 , 0 , 0 , 0 ] == 1 |

Table 3: Equations including the tokenized LaTeX input, the (optional) interpretation by Mathematica (Mat.), our translation (NMT), and the ground truth (GT.). (NMT+GT.) denotes that our translation is equal to the ground truth.

| | |
|---|---|
| | $$\sigma_k(2) = 1 + 2^k \quad \text{(B.6)}$$ |
| LaTeX | \sigma _ k ( 2 ) = 1 + 2 ^ k |
| Mat. | Subscript[\[Sigma], k][2] == 1 + 2^k |
| NMT+GT. | DivisorSigma [ k , 2 ] == 1 + 2 ^ k |
| | $$\int \sin(az) J_\nu(az) dz = \frac{z(az)_3^{1+\nu} F_4\left(\frac{3}{4}+\frac{\nu}{2}, 1+\frac{\nu}{2}, \frac{5}{4}+\frac{\nu}{2}; \frac{3}{2}, 2+\frac{\nu}{2}, 1+\nu, \frac{3}{2}+\nu; -a^2z^2\right)}{2^\nu((2+\nu)\Gamma(1+\nu))} \quad \text{(B.7)}$$ |
| LaTeX | **\int \sin ( a z ) J _ { \nu } ( a z ) d z** = \frac { z ( a z ) ^ { 1 + \nu } _ 3 F _ 4 \left( \frac { 3 } { 4 } + \frac { \nu } { 2 } , 1 + \frac { \nu } { 2 } , \frac { 5 } { 4 } + \frac { \nu } { 2 } ; \frac { 3 } { 2 } , 2 + \frac { \nu } { 2 } , 1 + \nu , \frac { 3 } { 2 } + \nu ; - a ^ 2 z ^ 2 \right) } { 2 ^ { \nu } ( ( 2 + \nu ) \Gamma ( 1 + \nu ) ) } |
| Mat. | Error; left half cannot be interpreted. Interpretation of right half: (z \!\(*SubsuperscriptBox[\(az\), \(3\), \(1 + \[Nu]\)]\) Subscript[F, 4][3/4 + \[Nu]/2, 1 + \[Nu]/2, 5/4 + \[Nu]/2; 3/2, 2 + \[Nu]/2, 1 + \[Nu], 3/2 + \[Nu]; -a^2 z^2])/(2^\[Nu] ((2 + \[Nu]) Gamma[1 + \[Nu]])) |
| NMT+GT. | **Integrate [ Sin [ a z ] BesselJ [ \[Nu] , a z ] , z ]** == ( z ( a z ) ^ ( 1 + \[Nu] ) HypergeometricPFQ [ { 3 / 4 + \[Nu] / 2 , 1 + \[Nu] / 2 , 5 / 4 + \[Nu] / 2 } , { 3 / 2 , 2 + \[Nu] / 2 , 1 + \[Nu] , 3 / 2 + \[Nu] } , ( - a ^ 2 ) z ^ 2 ] ) / 2 ^ \[Nu] / ( ( 2 + \[Nu] ) Gamma [ 1 + \[Nu] ] ) |
| | $$\wp(z; g_2, g_3) = \frac{1}{z^2} + \sum_{m=-\infty}^{\infty} \sum_{n=-\infty}^{\infty} \text{If}\left[\{m,n\} = \{0,0\}, 0, \frac{1}{(z-2m\omega_1-2n\omega_3)^2} - \frac{1}{(2m\omega_1+2n\omega_3)^2}\right] \quad \text{(B.8)}$$ |
| LaTeX | \wp \left( z ; g _ 2 , g _ 3 \right) = \frac { 1 } { z ^ 2 } + \sum _ { m = - \infty } ^ { \infty } \sum _ { n = - \infty } ^ { \infty } \text{If} \left[ \{ m , n \} = \{ 0 , 0 \} , 0 , \frac { 1 } { \left( z - 2 m \omega _ 1 - 2 n \omega _ 3 \right) { } ^ 2 } - \frac { 1 } { \left( 2 m \omega _ 1 + 2 n \omega _ 3 \right) { } ^ 2 } \right] |
| NMT+GT. | WeierstrassP [ z , { Subscript [ g , 2 ] , Subscript [ g , 3 ] } ] == 1 / z ^ 2 + Sum [ If [ { m , n } == { 0 , 0 } , 0 , 1 / ( z - 2 m Subscript [ \[Omega] , 1 ] - 2 n Subscript [ \[Omega] , 3 ] ) ^ 2 - 1 / ( 2 m Subscript [ \[Omega] , 1 ] + 2 n Subscript [ \[Omega] , 3 ] ) ^ 2 ] , { m , - Infinity , Infinity } , { n , - Infinity , Infinity } ] |

## C Qualitative Analysis – *semantic* LaTeX

This supplementary material presents and discusses 9 translation samples from LaTeX to *semantic* LaTeX. As before, all samples are randomly selected, only restricted by the editorial constraint of fitting on a single page and restricted to have a similar amount of exact matches and erroneous cases. Equations C.9–C.12 are erroneous translations, while Equations C.13–C.17 lead to exact matches.

In Equation C.9, our model accidentally outputs `\right) \right) }` instead of `} \right)` in the end of the equation. In Equation C.10, our model dropped the `i` after `\pi` because the input was `\pii`.

In Equation C.12, the symbol `\lambda` is just translated as `\lambda` instead of `\spheigvalLambda`. This might have happened since this is the only *semantic* LaTeX macro in the entire formula and the representation in the latent space might have caused not to translate this symbol into *semantic* LaTeX.

Table 4: Equations including the tokenized LaTeX input, our translation into *semantic* LaTeX (NMT), and the ground truth (GT.). (NMT+GT.) denotes that our translation is equal to the ground truth.

$$\Psi^{(\mathrm{E})}\left(\mathbf{x}\right) = 2\pi^2 \left(\frac{2}{3}\right)^{2/3} \sum_{n=0}^{\infty} \frac{\left(-i(2/3)^{2/3}z\right)^n}{n!} \Re\left(f_n\left(\frac{x+iy}{\texttt{<number\_24>}^{1/3}}, \frac{x-iy}{\texttt{<number\_24>}^{1/3}}\right)\right) \tag{C.9}$$

| | |
|---|---|
| LaTeX | \Psi ^ { ( \mathrm{E} ) } \left( \mathbf { x } \right) = 2 \pi ^ { 2 } \left( \dfrac { 2 } { 3 } \right) ^ { 2 / 3 } \sum \limits _ { n = 0 } ^ { \infty } \dfrac { \left( - i ( 2 / 3 ) ^ { 2 / 3 } z \right) ^ { n } } { n ! } \Re \left( f _ { n } \left( \dfrac { x + i y } { <number_24> ^ { 1 / 3 } } , \dfrac { x - i y } { <number_24> ^ { 1 / 3 } } \right) \right) |
| NMT | \ellumbcanonint @ { \mathbf { x } } = 2 \pi ^ { 2 } \left( \dfrac { 2 } { 3 } \right) ^ { 2 / 3 } \sum \limits _ { n = 0 } ^ { \infty } \dfrac { \left( - i ( 2 / 3 ) ^ { 2 / 3 } z \right) ^ { n } } { n ! } \realpart @ @ { \left( f _ { n } \left( \dfrac { x + i y } { <number_24> ^ { 1 / 3 } } , \dfrac { x - i y } { <number_24> ^ { 1 / 3 } } **} \right)** |
| GT. | \ellumbcanonint @ { \mathbf { x } } = 2 \pi ^ { 2 } \left( \dfrac { 2 } { 3 } \right) ^ { 2 / 3 } \sum \limits _ { n = 0 } ^ { \infty } \dfrac { \left( - i ( 2 / 3 ) ^ { 2 / 3 } z \right) ^ { n } } { n ! } \realpart @ @ { \left( f _ { n } \left( \dfrac { x + i y } { <number_24> ^ { 1 / 3 } } , \dfrac { x - i y } { <number_24> ^ { 1 / 3 } } **\right) \right) }** |

$$g(z) = e^{-\pi i/4}(2\sin\alpha)^{-1/2}\left(e^{-i\alpha}-z\right)^{-1/2} + e^{\pi i/4}(2\sin\alpha)^{-1/2}\left(e^{i\alpha}-z\right)^{-1/2} \tag{C.10}$$

| | |
|---|---|
| LaTeX | g ( z ) = e ^ { - \pi i / 4 } ( 2 \sin \alpha ) ^ { - 1 / 2 } \left( e ^ { - i \alpha } - z \right) ^ { - 1 / 2 } + e ^ { **\pii** / 4 } ( 2 \sin \alpha ) ^ { - 1 / 2 } \left( e ^ { i \alpha } - z \right) ^ { - 1 / 2 } |
| NMT | g ( z ) = e ^ { - \pi i / 4 } ( 2 \sin @ @ { \alpha } ) ^ { - 1 / 2 } \left( e ^ { - i \alpha } - z \right) ^ { - 1 / 2 } + e ^ { **\pi** / 4 } ( 2 \sin @ @ { \alpha } ) ^ { - 1 / 2 } \left( e ^ { i \alpha } - z \right) ^ { - 1 / 2 } |
| GT. | g ( z ) = e ^ { - \pi i / 4 } ( 2 \sin @ @ { \alpha } ) ^ { - 1 / 2 } \left( e ^ { - i \alpha } - z \right) ^ { - 1 / 2 } + e ^ { **\pi i** / 4 } ( 2 \sin @ @ { \alpha } ) ^ { - 1 / 2 } \left( e ^ { i \alpha } - z \right) ^ { - 1 / 2 } |

$$\Pi\left(\alpha^2,k\right) = \tfrac{\pi}{2}\sum_{n=0}^{\infty}\frac{\left(\tfrac{1}{2}\right)_n}{n!}\sum_{m=0}^{n}\frac{\left(\tfrac{1}{2}\right)_m}{m!}k^{2m}\alpha^{2n-2m} = \tfrac{\pi}{2}F_1\left(\tfrac{1}{2};\tfrac{1}{2},1;1;k^2,\alpha^2\right) \tag{C.11}$$

| | |
|---|---|
| LaTeX | \Pi \left( \alpha ^ { 2 } , k \right) = \frac { \pi } { 2 } \sum _ { n = 0 } ^ { \infty } \frac { { **\left( \tfrac { 1 } { 2 } \right) _ { n }** } } { n ! } \sum _ { m = 0 } ^ { n } \frac { { \left( \tfrac { 1 } { 2 } \right) _ { m } } } { m ! } k ^ { 2 m } \alpha ^ { 2 n - 2 m } = \frac { \pi } { 2 } { **F** _ { 1 } } \left( \tfrac { 1 } { 2 } ; \tfrac { 1 } { 2 } , 1 ; 1 ; k ^ { 2 } , \alpha ^ { 2 } \right) |
| NMT | \compellintPik @ { \alpha ^ { 2 } } { k } = \frac { \pi } { 2 } \sum _ { n = 0 } ^ { \infty } \frac { **\Pochhammersym { \tfrac { 1 } { 2 } } { n }** } { n ! } \sum _ { m = 0 } ^ { n } \frac { \Pochhammersym { \tfrac { 1 } { 2 } } { m } } { m ! } k ^ { 2 m } \alpha ^ { 2 n - 2 m } = \frac { \pi } { 2 } **\ge n h y p e r F** { 1 } { 1 } @ { \tfrac { 1 } { 2 } } { \tfrac { 1 } { 2 } , 1 } { k ^ { 2 } , \alpha ^ { 2 } } |
| GT. | \compellintPik @ { \alpha ^ { 2 } } { k } = \frac { \pi } { 2 } \sum _ { n = 0 } ^ { \infty } \frac { **\Pochhammersym { \tfrac { 1 } { 2 } } { n }** } { n ! } \sum _ { m = 0 } ^ { n } \frac { \Pochhammersym { \tfrac { 1 } { 2 } } { m } } { m ! } k ^ { 2 m } \alpha ^ { 2 n - 2 m } = \frac { \pi } { 2 } **\AppellF** { 1 } @ { \tfrac { 1 } { 2 } } { \tfrac { 1 } { 2 } } { 1 } { 1 } { k ^ { 2 } } { \alpha ^ { 2 } } |

Table 4: Equations including the tokenized LaTeX input, our translation into *semantic* LaTeX (NMT), and the ground truth (GT.). (NMT+GT.) denotes that our translation is equal to the ground truth.

| | |
|---|---|
| | $A_{-N-1}{a'}^{m}_{n,-N-2}(\gamma^2) + \left(B_{-N-1} - \lambda^{m}_{n}\left(\gamma^2\right)\right){a'}^{m}_{n,-N-1}(\gamma^2) + C'a^{m}_{n,-N}(\gamma^2) = 0$ (C.12) |
| LaTeX | A _ { - N - 1 } { a ^ { \prime } } ^ { m } _ { n , - N - 2 } ( \gamma ^ { 2 } ) + { \left( B _ { - N - 1 } - **\lambda** ^ { m } _ { n } \left( \gamma ^ { 2 } \right) \right) { a ^ { \prime } } ^ { m } _ { n , - N - 1 } ( \gamma ^ { 2 } ) } + C ^ { \prime } a ^ { m } _ { n , - N } ( \gamma ^ { 2 } ) = 0 |
| NMT | A _ { - N - 1 } { a ^ { \prime } } ^ { m } _ { n , - N - 2 } ( \gamma ^ { 2 } ) + { \left( B _ { - N - 1 } - **\lambda** ^ { m } _ { n } \left( \gamma ^ { 2 } \right) \right) { a ^ { \prime } } ^ { m } _ { n , - N - 1 } ( \gamma ^ { 2 } ) } + C ^ { \prime } a ^ { m } _ { n , - N } ( \gamma ^ { 2 } ) = 0 |
| GT. | A _ { - N - 1 } { a ^ { \prime } } ^ { m } _ { n , - N - 2 } ( \gamma ^ { 2 } ) + { \left( B _ { - N - 1 } - **\spheigvalLambda** { m } { n } @ { \gamma ^ { 2 } } \right) { a ^ { \prime } } ^ { m } _ { n , - N - 1 } ( \gamma ^ { 2 } ) } + C ^ { \prime } a ^ { m } _ { n , - N } ( \gamma ^ { 2 } ) = 0 |
| | $U_2(x,\alpha) = \frac{\pi^{1/2}m^{2/m}}{2^{(m+2)/(2m)}\Gamma(-1/m)}\left(W_m(t){-}W_m(-t)\right)$ (C.13) |
| LaTeX | U _ { 2 } ( x , \alpha ) = \frac { \pi ^ { 1 / 2 } m ^ { 2 / m } } { 2 ^ { ( m + 2 ) / ( 2 m ) } \Gamma \left( - 1 / m \right) } \left( W _ { m } ( t ) { - } W _ { m } ( - t ) \right) |
| NMT+GT. | U _ { 2 } ( x , \alpha ) = \frac { \pi ^ { 1 / 2 } m ^ { 2 / m } } { 2 ^ { ( m + 2 ) / ( 2 m ) } \EulerGamma @ { - 1 / m } } \left( W _ { m } ( t ) { - } W _ { m } ( - t ) \right) |
| | $(p_{\pm}^2 - p_{\mp}^2)R_J\left(x^2,y^2,z^2,p^2\right) = 2(p_{\pm}^2 - a^2)R_J\left(a^2,z_{+}^2,z_{-}^2,p_{\pm}^2\right) - 3R_F\left(x^2,y^2,z^2\right) + 3R_C\left(z^2,p^2\right)$ (C.14) |
| LaTeX | ( p _ { \pm } ^ { 2 } - p _ { \mp } ^ { 2 } ) R _ { J } \left( x ^ { 2 } , y ^ { 2 } , z ^ { 2 } , p ^ { 2 } \right) = 2 ( p _ { \pm } ^ { 2 } - a ^ { 2 } ) R _ { J } \left( a ^ { 2 } , z _ { + } ^ { 2 } , z _ { - } ^ { 2 } , p _ { \pm } ^ { 2 } \right) - 3 R _ { F } \left( x ^ { 2 } , y ^ { 2 } , z ^ { 2 } \right) + 3 R _ { C } \left( z ^ { 2 } , p ^ { 2 } \right) |
| NMT+GT. | ( p _ { \pm } ^ { 2 } - p _ { \mp } ^ { 2 } ) \CarlsonsymellintRJ @ { x ^ { 2 } } { y ^ { 2 } } { z ^ { 2 } } { p ^ { 2 } } = 2 ( p _ { \pm } ^ { 2 } - a ^ { 2 } ) \CarlsonsymellintRJ @ { a ^ { 2 } } { z _ { + } ^ { 2 } } { z _ { - } ^ { 2 } } { p _ { \pm } ^ { 2 } } - 3 \CarlsonsymellintRF @ { x ^ { 2 } } { y ^ { 2 } } { z ^ { 2 } } + 3 \CarlsonellintRC @ { z ^ { 2 } } { p ^ { 2 } } |
| | $a_n w_{n+1} - b_n w_n = d_n$ (C.15) |
| LaTeX | a _ { n } w _ { n + 1 } - b _ { n } w _ { n } = d _ { n } |
| NMT+GT. | a _ { n } w _ { n + 1 } - b _ { n } w _ { n } = d _ { n } |
| | $x = kr\,\operatorname{sn}\left(\beta,k\right)\operatorname{sn}\left(\gamma,k\right)$ (C.16) |
| LaTeX | x = k r \operatorname { s n } \left( \beta , k \right) \operatorname { s n } \left( \gamma , k \right) |
| NMT+GT. | x = k r \Jacobiellsnk @ { \beta } { k } \Jacobiellsnk @ { \gamma } { k } |

Table 4: Equations including the tokenized LaTeX input, our translation into *semantic* LaTeX (NMT), and the ground truth (GT.). (NMT+GT.) denotes that our translation is equal to the ground truth.

$$\frac{\mathrm{i}^{n}\mathrm{erfc}(z)}{\mathrm{i}^{n-1}\mathrm{erfc}(z)} = \cfrac{1/2}{z + \cfrac{(n+1)/2}{z + \cfrac{(n+2)/2}{z+}}} \cdots \tag{C.17}$$

| | |
|---|---|
| LaTeX | `\frac { \mathop { \mathrm{i} ^ { n } \mathrm{erfc} } \left( z \right) } { \mathop { \mathrm{i} ^ { n - 1 } \mathrm{erfc} } \left( z \right) } = \cfrac { 1 / 2 } { z + \cfrac { ( n + 1 ) / 2 } { z + \cfrac { ( n + 2 ) / 2 } { z + } } } \cdot s` |
| NMT+GT. | `\frac { \repinterfc { n } @ { z } } { \repinterfc { n - 1 } @ { z } } = \cfrac { 1 / 2 } { z + \cfrac { ( n + 1 ) / 2 } { z + \cfrac { ( n + 2 ) / 2 } { z + } } } \cdot s` |

## D Qualitative Analysis – im2latex-100k

This supplementary material presents and discusses 20 translation samples from LaTeX formulae published on arXiv to Mathematica. Given are only LaTeX expressions from the im2latex-100k data set. As before, all samples are randomly selected, only restricted to have a similar amount of exact matches and erroneous cases *as well as restricted to actually being equations*. Equations D.18–D.29 are exact match round trips, while the round trips of Equations D.30–D.37 require editing distances in the range of $15 - 30$.

Equation D.23 presumably uses the imaginary unit $i$. While our model interprets this as the Mathematica symbol for the imaginary unit (`I`), Mathematica interprets it as a variable (`i`).

Equation D.24 is an example of what would be considered very bad LaTeX style. Here, the comment "and cyclic" was written as $(andcyclic)$. Thus, it cannot be interpreted properly by our approach nor by Mathematica. Nevertheless, the round trips worked since it was just interpreted as one/multiple variable/s.

In Equation D.27, one of the six $A$s was mistakenly interpreted by our translator as the Glaisher-Kinkelin constant (`Glaisher`).

In Equation D.30, the sum $\sum_{k=l+1}^{N} \cdots$ was interpreted properly by Mathematica. Unfortunately, it mistakenly interprets the $B$ in $\sum_{k=l+1}^{N} q^{-m_0} B^{(N)}(L, r, l{+}1|k)$ as a `Beta` which is why the result of the round trip via our translator is: $\sum_{k}^{l+1} q^{-m_0} B_{(y,r)}(l+1, k)$. This is probably because the $N$ in $B^{(N)}$ confuses the network since the two spatially close symbols cause two very similar latent representations of $N$. This might have caused the cancellation of both $N$s.

In some of the recent samples, Mathematica's result was better since it does not try to interpret the equation's symbols. This is one of the major difficulties of trying to disambiguate mathematical formulae. If a data set of Mathematica expressions that contains fewer mathematically defined functions and more usages of variables and arbitrary functions denoted by the bare symbols existed, this would presumably prevent this issue.

Table 5: Equations including the tokenized LaTeX input, the interpretation by Mathematica (Mat.), and our translation (NMT).

| | | |
|---|---|---|
| | $\psi(x) = -2\phi(x) + 2\phi(L) + c$ | (D.18) |
| LaTeX | `\psi(x)=-2\phi(x)+2\phi(L)+c` | |
| Mat. | `\[Psi][x] == -2*\[Phi][x] + 2*\[Phi][L] + c` | |
| NMT | `PolyGamma[x] == - 2 EulerPhi[x] + 2 EulerPhi[L] + c` | |
| | $W(x) = \frac{x^3}{3} - a^2 x$ | (D.19) |
| LaTeX | `W(x)=\frac{x^3}{3}-a^2x` | |
| Mat. | `W[x] == x^3/3 - a^2*x` | |
| NMT | `ProductLog[x] == x ^ 3 / 3 - a ^ 2 x` | |
| | $f(\mu) = \pi - f(\pi - \mu)$ | (D.20) |
| LaTeX | `f(\mu)=\pi-f(\pi-\mu)` | |
| Mat. | `f[\[Mu]] == Pi - f[Pi - \[Mu]]` | |
| NMT | `f[\[Mu]] == Pi - f[Pi - \[Mu]]` | |
| | $\Delta(\varphi) = \varphi + \tilde{\varphi}$ | (D.21) |
| LaTeX | `\Delta(\varphi)=\varphi+\tilde{\varphi}` | |
| Mat. | `\[CapitalDelta][\[CurlyPhi]] == \[CurlyPhi] + OverTilde[\[CurlyPhi]]` | |
| NMT | `\[CapitalDelta][\[CurlyPhi]] == \[CurlyPhi] + OverTilde[\[CurlyPhi]]` | |
| | $\zeta(z) = \sum_{n=1}^{\infty} \frac{1}{n^z}$ | (D.22) |
| LaTeX | `\zeta(z)=\sum_{n=1}^{\infty}\frac{1}{n^z}` | |
| Mat. | `\[Zeta][z] == Sum[1/n^z, {n, 1, Infinity}]` | |
| NMT | `Zeta[z] == Sum[1 / n ^ z , { n , 1 , Infinity }]` | |
| | $\frac{1}{\sqrt{-i\pi(a-i\varepsilon)}}$ | (D.23) |
| LaTeX | `\frac{1}{\sqrt{-i\pi(a-i\varepsilon)}}` | |
| Mat. | `1/Sqrt[-i*Pi[a - i*\[Epsilon]]]` | |
| NMT | `1 / Sqrt[- I Pi ( a - I \[CurlyEpsilon] )]` | |
| | $ij = -ji = k(andcyclic)$ | (D.24) |
| LaTeX | `ij=-ji=k(andcyclic)` | |
| Mat. | `ij == -j*i == k[andcyclic]` | |
| NMT | `I j == - j I == k ( a n d c y c l I c )` | |
| | $\phi(x, y) = \lambda^{2s}\phi(\lambda x, \lambda y)$ | (D.25) |
| LaTeX | `\phi(x,y)=\lambda^{2s}\phi(\lambda x,\lambda y)` | |
| Mat. | `\[Phi][x, y] == \[Lambda]^(2*s)*\[Phi][Null, Null]` | |
| NMT | `EulerPhi[x , y] == \[Lambda] ^ ( 2 s ) EulerPhi[\[Lambda] x , \[Lambda] y]` | |

Table 5: Equations including the tokenized LaTeX input, the interpretation by Mathematica (Mat.), and our translation (NMT).

$$\varepsilon^{\lambda\mu m n}\varepsilon^{\sigma\nu p q}-\varepsilon^{\lambda\nu m n}\varepsilon^{\sigma\mu p q}=\varepsilon^{\sigma\lambda m n}\varepsilon^{\mu\nu p q} \tag{D.26}$$

LaTeX: \varepsilon^{\lambda\mu m n}\varepsilon^{\sigma\nu p q}-\varepsilon^{\lambda\nu m n}\varepsilon^{\sigma\mu p q}=\varepsilon^{\sigma\lambda m n}\varepsilon^{\mu\nu p q}

Mat.: \[Epsilon]^\[Lambda] * \[Epsilon]^\[Sigma] - \[Epsilon]^\[Lambda] * \[Epsilon]^\[Sigma] == \[Epsilon]^\[Sigma] * \[Epsilon]^\[Mu]

NMT: \[CurlyEpsilon] ^ ( \[Lambda] \[Mu] m n ) \[CurlyEpsilon] ^ ( \[Sigma] \[Nu] p q ) - \[CurlyEpsilon] ^ ( \[Lambda] \[Nu] m n ) \[CurlyEpsilon] ^ ( \[Sigma] \[Mu] p q ) == \[CurlyEpsilon] ^ ( \[Sigma] \[Lambda] m n ) \[CurlyEpsilon] ^ ( \[Mu] \[Nu] p q )

---

$$m_{A^1}=m_{A^2}=\sqrt{2}m_{A^4}=\sqrt{2}m_{A^5}=\sqrt{2}m_{A^6}=\sqrt{2}m_{A^7} \tag{D.27}$$

LaTeX: m_**{A**^1}=m_{A^2}=\sqrt{2}m_{A^4}=\sqrt{2}m_{A^5}=\sqrt{2}m_-{A^6}=\sqrt{2}m_{A^7}

Mat.: Subscript[m, **A**^1] == Subscript[m, A^2] == Sqrt[2]*Subscript[m, A^4] == Sqrt[2]*Subscript[m, A^5] == Sqrt[2]*Subscript[m, A^6] == Sqrt[2]*Subscript[m, A^7]

NMT: Subscript[m , **Glaisher** ^ 1] == Subscript[m , A ^ 2] == Sqrt[2] Subscript[m , A ^ 4] == Sqrt[2] Subscript[m , A ^ 5] == Sqrt[2] Subscript[m , A ^ 6] == Sqrt[2] Subscript[m , A ^ 7]

---

$$E_{37}=\{Q_1(x),Q_2(y)\}=-e^2(\alpha-1)\delta(x-y) \tag{D.28}$$

LaTeX: E_{37}=\{Q_1(x),Q_2(y)\}=-e^2(\alpha-1)\delta(x-y)

Mat.: Subscript[E, 37] == {Subscript[Q, 1][x], Subscript[Q, 2][y]} == -(e^2)[\[Alpha] - 1]*\[Delta][x - y]

NMT: EulerE[37] == { LegendreQ[1 , x] , LegendreQ[2 , y] } == - E ^ 2 ( \[Alpha] - 1 ) DiracDelta[x - y]

---

$$\lambda t K_{|n|}(\mu t)I_{|n|}(\mu t) \tag{D.29}$$

LaTeX: \lambda t K_{\left|n\right|}(\mu t)I_{\left|n\right|}(\mu t)

Mat.: Error

NMT: \[Lambda] t BesselK[Abs[n] , \[Mu] t] BesselI[Abs[n] , \[Mu] t]

---

$$q^{(\frac{L}{2}-\frac{r}{N})}\sum_{k=l+1}^N q^{-m_0}B^{(N)}(L,r,l+1|k)=\sum_{k=l+1}^N B^{(N)}(L,r,l|k) \tag{D.30}$$

LaTeX: q^{(\frac{L}{2}-\frac{r}{N})}\sum_{k=l+1}^Nq^{-m_0}B^{(N)}(L,r,l+1|k)= **\sum_{k=l+1}^N**B^{(N)}(L,r,l|k)

Mat.: q^(L/2 - r/N)***Sum[**(B^N)[L, r, l + 1 | k]/q^Subscript[m, 0]**, {k == l + 1, N}]** == Sum[(B^N)[L, r, l | k], {k == l + 1, N}]

NMT: q ^ ( L / 2 - r / q ) **Sum[**q ^ ( - Subscript[m , 0] ) Beta[y , r , l + 1 , k] **, { k , l + 1 }]** == Sum[B[LaguerreL[r , l , k] , r , l , k] , { k , l + 1 , 1 }]

---

$$\gamma_1=-\gamma-1-\gamma(-2-a-b)-\delta(2-a/\delta-b/\delta-2a-2b)-9/139(1+a+b) \tag{D.31}$$

LaTeX: \gamma_1=-\gamma-1-\gamma(-2-a-b)- \delta (2-a/\delta-b/\delta-2a-2b)-9/139(1+a+b)

Mat.: Subscript[\[Gamma], 1] == -\[Gamma] - 1 - \[Gamma][-2 - a - b] - \[Delta][2 - a/\[Delta] - b/\[Delta] - 2*a - 2*b] - 9/139*(1 + a + b)

NMT: StieltjesGamma[1] == - EulerGamma - 1 - EulerGamma ( - 2 - a - b ) - DiracDelta[2 - a / DiracDelta - b] - 9 / ( 1 + a + b )

Table 5: Equations including the tokenized LaTeX input, the interpretation by Mathematica (Mat.), and our translation (NMT).

| | | |
|---|---|---|
| | $$I_n(x) = \int_0^x dx_n \int_0^{x_n} dx_{n-1} \cdots \int_0^{x_2} dx_1 \cdot 1 = \frac{x^n}{n!}$$ | (D.32) |
| LaTeX | `I_n(x)=\int_0^xdx_n\int_0^{x_n}dx_{n-1}\cdots\int_0^{x_2}dx_-1\cdot1=\frac{x^n}{n!}` | |
| Mat. | `Error` | |
| NMT | `BesselI[n , x] == Integrate[d Subscript[x , n] Integrate[Subscript[x , n] , { Subscript[x , n] , 0 , Subscript[x , n] }] , { Subscript[x , n] , 0 , Subscript[x , n] }] == ( x ^ n / n ! )` | |
| | $$L_4^g = \frac{1}{4} I_4 - I_7$$ | (D.33) |
| LaTeX | `L^g_4=\frac{1}{4}I_4-I_7` | |
| Mat. | `Subscript[L, 4]^g == 1/4*Subscript[I, 4] - Subscript[I, 7]` | |
| NMT | `LucasL[4] == ( 1 / 4 ) BesselI[4] - BesselI[7]` | |
| | $$\frac{d\lambda^\gamma}{du} = \tilde{f}_\gamma(u)\lambda_1$$ | (D.34) |
| LaTeX | `\frac{d\lambda^{\gamma}}{du}={\tilde f}_{\gamma}(u)\lambda_1` | |
| Mat. | `(d*\[Lambda]^\[Gamma])/du == Subscript[\[Null], \[Gamma]][u]*Subscript[\[Lambda], 1]` | |
| NMT | `( d \[Lambda] ^ \[Gamma] ) / ( d u ) == ( u ) Subscript[\[Lambda] , 1]` | |
| | $$k^2 = \frac{b^2}{4} + \frac{\pi^2}{y_c^2} n_k^2$$ | (D.35) |
| LaTeX | `k^2=\frac{b^2}{4}+\frac{\pi^2}{y_c^2}n_k^2` | |
| Mat. | `k^2 == b^2/4 + Pi^2/Subscript[y, c]^2*Subscript[n, k]^2` | |
| NMT | `k ^ 2 == b ^ 2 / 4 + Pi ^ 2 / Subscript[y , c] ^ 2 Subscript[n , k] ^ 2` | |
| | $$S = trH^4 - 2\mu^2 trH^2 + n\mu^4$$ | (D.36) |
| LaTeX | `S=trH^{4}-2{\mu}^{2}trH^{2}+n{\mu}^{4}` | |
| Mat. | `S == t*r*H^4 - 2*\[Mu]^2*t*r*H^2 + n*\[Mu]^4` | |
| NMT | `FresnelS[t r / 4 - 2 / \[Mu] , r] ^ 2 + n / \[Mu] ^ 4` | |
| | $$S^{-1}(p) = i\gamma \cdot pA(p^2) + B(p^2)$$ | (D.37) |
| LaTeX | `S^{-1}(p)=i\gamma\cdot pA(p^{2})+B(p^{2})` | |
| Mat. | `(S^(-1))[p] == i*\[Gamma][p^2] + B[p^2]` | |
| NMT | `StirlingS1[p , p] == I EulerGamma ï PartitionsP[p ^ 2]+Beta[p^2]` | |
